# Supplementary material for: Network Traffic Dynamics in Urban Low-Altitude Air Transport with Projected-Space Macroscopic Fundamental Diagrams
Source: arXiv:2611.27357 source file (2026-11-20)
Supplement: Supplementary file 4 [file app4_largetables.tex]

\section{Supplementary numerical results}
\label{app:numerical_results}

\subsection{Aggregate outflow estimation statistics}
\label{app:outflow_statistics}

\autoref{tab:multiclass_outflow_statistics} provides detailed numerical results supporting the aggregate multi-class MFD verification in \autoref{subsubsec:mc_verification}, for generation priority fractions $\alpha_{\mathrm{pr}}^q\in\{0.2,0.4,0.6,0.8\}$. The table reports the mean and standard deviation of the observed outflow $G_0$ and the projected-space estimate $\hat G_{\mathrm{AB}}^{\mathrm{proj}}$ across multiple independent simulation runs. For compactness, we denote their means by $\mu_0=\mu(G_0)$ and $\hat\mu=\mu(\hat G_{\mathrm{AB}}^{\mathrm{proj}})$, and their standard deviations by $\sigma_0=\sigma(G_0)$ and $\hat\sigma=\sigma(\hat G_{\mathrm{AB}}^{\mathrm{proj}})$. The signed relative estimation error is defined as
\begin{equation}
    \epsilon_G =
    \frac{
        \mu(\hat G_{\mathrm{AB}}^{\mathrm{proj}})-\mu(G_0)
    }{
        \mu(G_0)
    }\times 100\%.
\end{equation}
All statistics are computed from the unrounded data and reported to three decimal places. The first column uses standardized accumulation-level labels corresponding to the progressive-loading stages.

\begin{table}[pos = htbp]
    \centering
    \caption{Observed and estimated aggregate outflow statistics for different generation priority fractions. Means and standard deviations are expressed in [a.c./s], and $\epsilon_G$ denotes the signed relative estimation error in [\%].}
    \label{tab:multiclass_outflow_statistics}

    \begingroup
    \fontsize{9}{10.5}\selectfont
    \setlength{\tabcolsep}{2pt}
    \renewcommand{\arraystretch}{1.05}

    \begin{minipage}[t]{0.49\linewidth}
        \centering
        $\alpha_{\mathrm{pr}}^q=0.2$\par
        \smallskip
        \begin{tabular}{@{}rrrrrr@{}}
            \toprule
            $n$ & $\mu_0$ & $\hat\mu$ & $\epsilon_G$ & $\sigma_0$ & $\hat\sigma$ \\
            \midrule
              1 & 0.028 & 0.030 & 6.731 & 0.002 & 0.003 \\
             21 & 0.559 & 0.561 & 0.255 & 0.010 & 0.009 \\
             41 & 1.035 & 1.038 & 0.269 & 0.008 & 0.010 \\
             61 & 1.447 & 1.448 & 0.092 & 0.015 & 0.014 \\
             81 & 1.804 & 1.806 & 0.118 & 0.022 & 0.022 \\
            101 & 2.120 & 2.121 & 0.040 & 0.021 & 0.020 \\
            121 & 2.338 & 2.340 & 0.108 & 0.031 & 0.030 \\
            141 & 2.440 & 2.441 & 0.052 & 0.080 & 0.079 \\
            161 & 2.059 & 2.058 & -0.058 & 0.349 & 0.343 \\
            181 & 1.079 & 1.090 & 1.027 & 0.215 & 0.220 \\
            201 & 0.656 & 0.672 & 2.573 & 0.090 & 0.091 \\
            221 & 0.418 & 0.430 & 2.995 & 0.112 & 0.110 \\
            241 & 0.279 & 0.294 & 5.263 & 0.065 & 0.069 \\
            261 & 0.212 & 0.226 & 6.310 & 0.047 & 0.048 \\
            281 & 0.160 & 0.173 & 8.378 & 0.033 & 0.032 \\
            301 & 0.143 & 0.168 & 17.320 & 0.047 & 0.045 \\
            \bottomrule
        \end{tabular}
    \end{minipage}%
    \hfill
    \begin{minipage}[t]{0.49\linewidth}
        \centering
        $\alpha_{\mathrm{pr}}^q=0.4$\par
        \smallskip
        \begin{tabular}{@{}rrrrrr@{}}
            \toprule
            $n$ & $\mu_0$ & $\hat\mu$ & $\epsilon_G$ & $\sigma_0$ & $\hat\sigma$ \\
            \midrule
              1 & 0.028 & 0.030 & 7.257 & 0.001 & 0.003 \\
             21 & 0.557 & 0.558 & 0.224 & 0.012 & 0.011 \\
             41 & 1.034 & 1.034 & -0.018 & 0.010 & 0.010 \\
             61 & 1.457 & 1.456 & -0.058 & 0.016 & 0.015 \\
             81 & 1.828 & 1.832 & 0.215 & 0.018 & 0.018 \\
            101 & 2.170 & 2.170 & 0.028 & 0.018 & 0.019 \\
            121 & 2.421 & 2.422 & 0.043 & 0.034 & 0.036 \\
            141 & 2.608 & 2.612 & 0.159 & 0.047 & 0.048 \\
            161 & 2.761 & 2.763 & 0.099 & 0.072 & 0.074 \\
            181 & 2.559 & 2.560 & 0.019 & 0.342 & 0.342 \\
            201 & 1.793 & 1.796 & 0.180 & 0.429 & 0.425 \\
            221 & 1.082 & 1.100 & 1.660 & 0.178 & 0.173 \\
            241 & 0.711 & 0.731 & 2.729 & 0.142 & 0.139 \\
            261 & 0.498 & 0.514 & 3.157 & 0.105 & 0.113 \\
            281 & 0.380 & 0.398 & 4.545 & 0.081 & 0.082 \\
            301 & 0.249 & 0.272 & 9.128 & 0.045 & 0.044 \\
            \bottomrule
        \end{tabular}
    \end{minipage}

    \par\vspace{0.8em}

    \begin{minipage}[t]{0.49\linewidth}
        \centering
        $\alpha_{\mathrm{pr}}^q=0.6$\par
        \smallskip
        \begin{tabular}{@{}rrrrrr@{}}
            \toprule
            $n$ & $\mu_0$ & $\hat\mu$ & $\epsilon_G$ & $\sigma_0$ & $\hat\sigma$ \\
            \midrule
              1 & 0.029 & 0.030 & 4.882 & 0.002 & 0.003 \\
             21 & 0.560 & 0.561 & 0.241 & 0.012 & 0.011 \\
             41 & 1.040 & 1.039 & -0.046 & 0.008 & 0.008 \\
             61 & 1.456 & 1.458 & 0.111 & 0.018 & 0.016 \\
             81 & 1.834 & 1.832 & -0.079 & 0.016 & 0.015 \\
            101 & 2.158 & 2.159 & 0.020 & 0.019 & 0.021 \\
            121 & 2.442 & 2.445 & 0.112 & 0.036 & 0.036 \\
            141 & 2.665 & 2.666 & 0.031 & 0.034 & 0.035 \\
            161 & 2.853 & 2.855 & 0.055 & 0.035 & 0.036 \\
            181 & 2.994 & 2.992 & -0.042 & 0.039 & 0.042 \\
            201 & 3.035 & 3.036 & 0.053 & 0.098 & 0.096 \\
            221 & 2.915 & 2.913 & -0.074 & 0.169 & 0.169 \\
            241 & 2.579 & 2.583 & 0.153 & 0.198 & 0.190 \\
            261 & 2.082 & 2.087 & 0.271 & 0.281 & 0.276 \\
            281 & 1.623 & 1.638 & 0.926 & 0.199 & 0.193 \\
            301 & 1.165 & 1.206 & 3.474 & 0.153 & 0.159 \\
            \bottomrule
        \end{tabular}
    \end{minipage}%
    \hfill
    \begin{minipage}[t]{0.49\linewidth}
        \centering
        $\alpha_{\mathrm{pr}}^q=0.8$\par
        \smallskip
        \begin{tabular}{@{}rrrrrr@{}}
            \toprule
            $n$ & $\mu_0$ & $\hat\mu$ & $\epsilon_G$ & $\sigma_0$ & $\hat\sigma$ \\
            \midrule
              1 & 0.028 & 0.029 & 4.162 & 0.001 & 0.002 \\
             21 & 0.564 & 0.564 & 0.008 & 0.009 & 0.009 \\
             41 & 1.030 & 1.030 & 0.064 & 0.010 & 0.012 \\
             61 & 1.439 & 1.439 & -0.013 & 0.015 & 0.016 \\
             81 & 1.808 & 1.810 & 0.083 & 0.012 & 0.016 \\
            101 & 2.117 & 2.120 & 0.185 & 0.016 & 0.014 \\
            121 & 2.369 & 2.369 & -0.024 & 0.019 & 0.015 \\
            141 & 2.591 & 2.594 & 0.117 & 0.047 & 0.050 \\
            161 & 2.723 & 2.726 & 0.123 & 0.041 & 0.039 \\
            181 & 2.630 & 2.630 & 0.003 & 0.335 & 0.329 \\
            201 & 2.004 & 2.017 & 0.622 & 0.758 & 0.750 \\
            221 & 1.055 & 1.074 & 1.806 & 0.454 & 0.452 \\
            241 & 0.549 & 0.573 & 4.259 & 0.164 & 0.165 \\
            261 & 0.307 & 0.329 & 7.069 & 0.099 & 0.099 \\
            281 & 0.216 & 0.232 & 7.407 & 0.080 & 0.081 \\
            301 & 0.174 & 0.204 & 16.921 & 0.033 & 0.035 \\
            \bottomrule
        \end{tabular}
    \end{minipage}

    \endgroup
\end{table}
